# Supplementary material for: Evolving Microstructures in Relaxed Continuum Damage Mechanics for Strain Softening
Source: arXiv:2208.14695 source file (2022-08-31)
Supplement: Supplementary file 1 [file sec_appendix.tex]

\section{This is a first Appendix \label{app:A}} 

This is the text of the first appendix. 

\section{This is the second Appendix}

This is the second appendix, the first one is given in Appendix~\ref{app:A}.
